# Supplementary material for: Degree Four Plane Spanners: Simpler and Better
Source: arXiv:1603.03818 source file (2016-03-11)
Supplement: Supplementary file 1 [file appendix.tex]

\section{Appendix}
